# Supplementary material for: Strong Amplitude and Phase Modulation of Optical Spatial Coherence with Surface Plasmon Polaritons
Source: arXiv:1612.09153 ancillary file (2016-12-29)
Supplement: Supplementary file 1 [file SupplementaryMaterials.pdf]

# Strong Amplitude and Phase Modulation of Optical Spatial Coherence with Surface Plasmon Polaritons

Dongfang Li and Domenico Pacifici*
*School of Engineering, Brown University, Providence, Rhode Island, 02912, United States*

## Materials and Methods

**Fabrication of Young's double-slit interferometers.** Electron beam evaporation was employed to deposit an ~200nm-thick layer of silver (Ag) on one of the two surfaces of a 1mm-thick glass slide that was previously coated with a 3nm-thick titanium (Ti) layer to improve film adhesion. Multiple Young's double-slit interferometers, consisting of two identical ~200nm-wide, ~200nm-deep and ~15$\mu$m-long through-slits, with variable slit-slit separation distance, were etched on the silver film using focused ion beam (FIB) milling (see Fig. S2). The separation distance between the two slits ranged from 0.5 $\mu$m to 9.525 $\mu$m in incremental steps of 25 nm. In total, 362 Young's double-slit interferometers were etched on the metal film, evenly distributed in two separate columns. A single column containing 181 identical individual slits was also etched on the same silver film to serve as reference to normalize light transmission through double-slits. The columns of single- or double-slits were placed 600 $\mu$m apart, and adjacent slits along each column were separated by 25 $\mu$m to avoid optical cross-talk during the measurements that could affect the interference patterns and lead to artificially reduced visibility values.

**Optical characterization setup.** Köhler illumination was employed to achieve variable spatial coherence illumination of Young's double-slit interferometers. The setup consisted of a xenon arc lamp, coupled to an inverted microscope, together with a diffuser, an auxiliary lens, a linear polarizer, a 2mm-wide slit mask, and a condenser lens system [1]. Each interferometer was illuminated from the glass side –i.e. from glass(1 mm)/Ti(3 nm)/Ag(200 nm) interface– and the transmitted light intensity was collected with a 20× objective (0.75 numerical aperture) from the opposite side, that is from the Ag(200 nm)/air interface. The focal plane of the objective lens was located ~49 $\mu$m below the metal surface containing the double-slit interferometers to generate far-zone projections of light intensity onto the imaging plane of a charged coupled device (CCD) camera. More specifically, the interference pattern was projected onto the entrance slit mask of a spectrograph, dispersed by a grating with 150 grooves/mm, and imaged onto a two-dimensional CCD camera to extract the wavelength dependence of light intensity along the horizontal axis and the spatial intensity distribution along the vertical axis (see Fig. 1 in main text). This experimental setup allows detection of wavelength-resolved interference patterns transmitted through each Young's double-slit interferometer, from which the fringe visibility over several wavelengths can be captured simultaneously in a single CCD image. By scanning all of the double-slit interferometers with different separation distances using an automated microscope stage, 362 wavelength-resolved interference patterns were obtained for each subtended angle, and for TE (i.e., no surface plasmon polaritons, SPPs) or TM (i.e., with SPPs) polarization states of the incident light (see Fig. S3). Additionally, a full set of light transmission experiment was also performed for all the double-slits and reference single-slits by focusing the microscope objective directly onto the output metal film surface, in order to measure plasmonic interferograms necessary to determine SPP excitation, propagation, and coupling coefficients for both top (glass/Ti/Ag) and bottom (Ag/air) interfaces as a function of incident wavelength. Note that a Nikon Perfect Focus System was employed during the scanning process to keep a constant relative distance between the microscope objective and the bottom sample surface (i.e., Ag/air interface).

**Calculations of surface plasmon polariton refractive index and wavevector.** The wavevectors of SPPs propagating along the top (glass/Ti/Ag, with $k_{\mathrm{SPP,t}} = n_{\mathrm{SPP,t}} k_0$) and bottom (Ag/air, with $k_{\mathrm{SPP,b}} = n_{\mathrm{SPP,b}} k_0$) metal/dielectric interfaces were calculated and compared with the experimental data extracted from plasmonic interferograms and Fourier transform analysis. Specifically, $n_{\mathrm{SPP,t}}$ was calculated by employing a finite-difference frequency-domain (FDFD) numerical method adapted to a three-layer system [2], whereas $n_{\mathrm{SPP,b}} = \sqrt{\epsilon_{\mathrm{Ag}}\epsilon_{\mathrm{air}}/(\epsilon_{\mathrm{Ag}} + \epsilon_{\mathrm{air}})}$, with $\epsilon_{\mathrm{Ag}}$ and $\epsilon_{\mathrm{air}}$ the dielectric functions of silver and air, respectively. In all calculations, the dielectric function of silver was measured by variable angle spectroscopic ellipsometry (VASE) on a freshly deposited film, the refractive index of titanium was obtained from tabulated data [3], and a constant refractive index of 1.43 was assumed for glass.

**Data analysis of interference patterns.** All interference patterns (Figs. 1,2,4 and Figs. S3,S6) were normalized to the corresponding mean intensity value at each wavelength to remove the wavelength-dependent intensity variation

*Electronic address: Domenico_Pacifici@brown.edu

introduced by the external light source and enforce the similar intensity range for all interference patterns, so that they could be clearly plotted together on the same color map.

**Variable spatial coherence (Köhler) illumination of Young's double-slit interferometers.** Under Köhler illumination, linearly-polarized electromagnetic fields incident upon the sample surface with the same angle of incidence $\theta$ (that is, the same wavevector) can be summed up coherently, since they originate from the same point-like light source. Therefore, for any given angle of incidence $\theta$, the TE electric fields projected from each slit onto a screen, reaching a point located a distance $x$ from the central (slit-slit) axis can be expressed using complex notation as (see Fig. S1 for a schematic of the experiment):

$$E_{\mathrm{TE},1}(x,\theta) = E_{0,1}(x)e^{ik_0 l_1}, \quad E_{\mathrm{TE},2}(x,\theta) = E_{0,2}(x)e^{ik_0 d\sin\theta}e^{ik_0 l_2}, \tag{S1}$$

$$E_{0,\mathrm{j}}(x) = E_0 \frac{\sin(\pi w \frac{\sin\alpha_\mathrm{j}}{\lambda})}{\pi w \frac{\sin\alpha_\mathrm{j}}{\lambda}}, \tag{S2}$$

where $j = 1, 2$, $\alpha_1(x) = \tan^{-1}[(x + d/2)/D]$ and $\alpha_2(x) = \tan^{-1}[(x - d/2)/D]$, $d$ is the center-to-center slit-slit separation distance, $D$ is the distance between the projection screen and the plane containing the double-slits, $w$ is the effective width of each slit whose value can be extracted by fitting the single-slit experimental diffraction pattern to Eq. (S2) using $d = 0$ (see Fig. S4), $l_1 = \sqrt{D^2 + (x + d/2)^2}$ and $l_2 = \sqrt{D^2 + (x - d/2)^2}$, $E_0$ is the electric field amplitude at the central location of the single-slit diffraction pattern on the projection screen, $E_{0,\mathrm{j}}(x)$ is the amplitude of the electric field projected onto the screen at position $x$ from slit $j$, which is independent of incident angle $\theta$ for the sub-wavelength-width slit employed in this work (see Fig. S4). Note that Snell's law requires that $\sin\theta = n\sin\theta'$ (Fig. S1), with $n$ the refractive index of the substrate supporting the metal film. The interference pattern for a specific angle of incidence $\theta$ (i.e., $I_{\mathrm{TE}}(x,\theta)$, thin gray lines labeled as $\theta = 0°$ to $5°$ in Fig. S1) under TE-polarized illumination can be written as:

$$I_{\mathrm{TE}}(x,\theta) = |E_{\mathrm{TE},1}(x,\theta) + E_{\mathrm{TE},2}(x,\theta)|^2. \tag{S3}$$

In contrast, incident light from different angles can be treated as totally incoherent. While illuminating Young's double-slit interferometer with a subtended angle $\Delta\theta$ (i.e., $\theta$ varying from $-\Delta\theta/2$ to $\Delta\theta/2$), the interference pattern (e.g., shaded gray area in Fig. S1), including single-slit diffraction effects, can be expressed as:

$$I_{\mathrm{TE},\Delta\theta}(x) = \frac{1}{\Delta\theta}\int_{-\Delta\theta/2}^{\Delta\theta/2} I_{\mathrm{TE}}(x,\theta)d\theta. \tag{S4}$$

The reference interference pattern (thick gray line in Fig. S1) is calculated from $I_{\mathrm{Ref}}(x) = |E_{0,1}(x)|^2 + |E_{0,2}(x)|^2$.

However, when the polarization of the incident light is changed from TE to TM, SPP contributions from each slit are turned on, which can mix the electromagnetic fields incident on each of the double-slits, and therefore modulate the interference patterns projected on the screen. The electric fields on the top and bottom of the double-slits can be written as:

$$E_{\mathrm{TM,t1}}(\theta) = E_{\mathrm{TM,t01}} + E_{\mathrm{TM,t02}}\beta_\mathrm{t}e^{ik_{\mathrm{SPP,t}}d}, \quad E_{\mathrm{TM,t2}}(\theta) = E_{\mathrm{TM,t02}} + E_{\mathrm{TM,t01}}\beta_\mathrm{t}e^{ik_{\mathrm{SPP,t}}d}, \tag{S5}$$

$$E_{\mathrm{TM,b1}}(\theta) = \tau E_{\mathrm{TM,t1}} + \tau E_{\mathrm{TM,t2}}\beta_\mathrm{b}e^{ik_{\mathrm{SPP,b}}d}, \quad E_{\mathrm{TM,b2}}(\theta) = \tau E_{\mathrm{TM,t1}}\beta_\mathrm{b}e^{ik_{\mathrm{SPP,b}}d} + \tau E_{\mathrm{TM,t2}}, \tag{S6}$$

where $E_{\mathrm{TM,t01}}$ and $E_{\mathrm{TM,t02}}$ are the electric fields originally incident on the double-slit locations, $\beta_\mathrm{t}$ and $\beta_\mathrm{b}$ refer to the SPPs coupling coefficients at the top (i.e., glass/Ti/Ag) and bottom interface (i.e., Ag/air), $k_{\mathrm{SPP,t}}$ and $k_{\mathrm{SPP,b}}$ are the corresponding complex wavevectors of SPPs, $\tau$ is the transmission coefficient through each slit. Using the relation $E_{\mathrm{TM,t02}} = E_{\mathrm{TM,t01}}e^{ik_0 d\sin\theta}$ (see Fig. S1), Eq. (S5) can be expressed as:

$$E_{\mathrm{TM,t1}}(\theta) = E_{\mathrm{TM,t01}}(1 + \beta_\mathrm{t}e^{ik_{\mathrm{SPP,t}}d}e^{ik_0 d\sin\theta}), \quad E_{\mathrm{TM,t2}}(\theta) = E_{\mathrm{TM,t01}}(e^{ik_0 d\sin\theta} + \beta_\mathrm{t}e^{ik_{\mathrm{SPP,t}}d}). \tag{S7}$$

By applying Eq. (S7) to Eq. (S6), the electric fields on the bottom interface can be expressed as:

$$E_{\mathrm{TM,b1}}(\theta) = \tau E_{\mathrm{TM,t01}}(1 + \beta e^{ik_0 d\sin\theta} + \beta_\mathrm{t}\beta_\mathrm{b}e^{i(k_{\mathrm{SPP,t}}+k_{\mathrm{SPP,b}})d}), \tag{S8}$$

$$E_{\mathrm{TM,b2}}(\theta) = \tau E_{\mathrm{TM,t01}}(\beta + e^{ik_0 d\sin\theta} + \beta_\mathrm{t}\beta_\mathrm{b}e^{i(k_{\mathrm{SPP,t}}+k_{\mathrm{SPP,b}})d}e^{ik_0 d\sin\theta}), \tag{S9}$$

where $\beta = \beta_\mathrm{t}e^{ik_{\mathrm{SPP,t}}d} + \beta_\mathrm{b}e^{ik_{\mathrm{SPP,b}}d}$ is a wavelength-dependent SPP coupling coefficient including both interfaces. By neglecting the higher-order contributions (i.e., the third term $\beta_\mathrm{t}\beta_\mathrm{b}e^{i(k_{\mathrm{SPP,t}}+k_{\mathrm{SPP,b}})d}$ and $\beta_\mathrm{t}\beta_\mathrm{b}e^{i(k_{\mathrm{SPP,t}}+k_{\mathrm{SPP,b}})d}e^{ik_0 d\sin\theta}$) in Eqs. (S8) and (S9), these equations can be simplified as follows:

$$E_{\mathrm{TM,b1}}(\theta) \approx \tau E_{\mathrm{TM,t01}}(1 + \beta e^{ik_0 d\sin\theta}), \quad E_{\mathrm{TM,b2}}(\theta) \approx \tau E_{\mathrm{TM,t01}}(\beta + e^{ik_0 d\sin\theta}). \tag{S10}$$

Thus, the electric fields projected onto the screen at position $x$ under TM-polarized illumination can be expressed as:

$$E_{\mathrm{TM},1}(x,\theta) \approx (1+\beta e^{ik_0 d\sin\theta})E_{0,1}(x)e^{ik_0 l_1}, \quad E_{\mathrm{TM},2}(x,\theta) \approx (\beta + e^{ik_0 d\sin\theta})E_{0,2}(x)e^{ik_0 l_2}, \tag{S11}$$

where $E_{0,\mathrm{j}}(x)$ is the amplitude of the electric fields projected onto the screen at position $x$ originating from slit $j$ with output field amplitude $\tau E_{\mathrm{TM,t01}}$ at the slit location.

The corresponding interference pattern under a fixed angle $\theta$ or a subtended angle $\Delta\theta$ can be expressed as:

$$I_{\mathrm{TM}}(x,\theta) = |E_{\mathrm{TM},1}(x,\theta) + E_{\mathrm{TM},2}(x,\theta)|^2, \tag{S12}$$

$$I_{\mathrm{TM},\Delta\theta}(x) = \frac{1}{\Delta\theta}\int_{-\Delta\theta/2}^{\Delta\theta/2} I_{\mathrm{TM}}(x,\theta)d\theta. \tag{S13}$$

The degree of spatial coherence can be extracted from the interference pattern calculated by Eqs. (S4) and (S13) for TE- and TM-polarized illumination, respectively. The calculated results of SPP-induced spatial coherence modulation are in good agreement with the developed analytical model [4, 5] (see Fig. S5) and the experimental data (see Fig. S6).

**Extraction of SPP coupling coefficients from plasmonic interferograms.** The light spectra transmitted through double-slits ($I_{\mathrm{DS}}$) and reference single-slits ($I_{\mathrm{SS}}$) were measured by focusing the objective onto the nanoapertures. The scalar field transmitted through the single-slit ($E_{\mathrm{SS}}$) and double-slit ($E_{\mathrm{DS}}$) can be expressed as follows:

$$E_{\mathrm{SS}}(\lambda) = \tau E_{\mathrm{in}}(\lambda), \tag{S14}$$

$$E_{\mathrm{DS}}(\lambda, d) = \tau E_{\mathrm{in}}(\lambda) + \tau\beta E_{\mathrm{in}}(\lambda), \tag{S15}$$

where the field incident on each slit is assumed to be the same ($E_{\mathrm{in}}$) and the two incident fields on the slits can be considered fully coherent up to 5 $\mu$m separation distance under subtended illumination angle $\Delta\theta \approx 3°$ (corresponding to $\mu_{\mathrm{in}} \geq 0.7$). Accordingly, the normalized intensity ratio of the transmitted intensity through the double-slit and the reference single-slit can be written as:

$$I_{\mathrm{n}}(\lambda, d) = \frac{I_{\mathrm{DS}}(\lambda, d)}{2I_{\mathrm{SS}}(\lambda)} = \frac{\langle E^*_{\mathrm{DS}}E_{\mathrm{DS}}\rangle}{\langle E^*_{\mathrm{SS}}E_{\mathrm{SS}}\rangle} = |1+\beta|^2 = |1+\beta_{\mathrm{t}}e^{ik_{\mathrm{SPP,t}}d} + \beta_{\mathrm{b}}e^{ik_{\mathrm{SPP,b}}d}|^2, \tag{S16}$$

where the factor 2 in the denominator arises from the fact that the two slits in the Young's double-slit interferometer can be fully distinguished by the optical setup, therefore the intensity (rather than the fields) can be summed up when the two slits are directly imaged.

A representative plasmonic interferogram at wavelength 600 nm is plotted in Fig. 3A (black line). The wavelength-resolved plasmonic interferograms are shown in Fig. 3C. Applying discrete Fourier transform to the plasmonic interferograms, different orders of SPP contributions can be deconvolved [1, 6], as shown by the peaks and bright bands in Fig. 3B,D, which are in good agreement with the calculated wavevectors of different orders of SPP (grays lines in Fig. 3D). SPP contributions from both interfaces (black *vs.* red labels) are clearly evidenced. After filtering out higher-order SPP contributions (i.e., with $m > 1$), plasmonic interferograms that only originate from first-order SPPs can be reconstructed (red line in Fig. 3A). By fitting the reconstructed plasmonic interferograms (with $d$ ranging from 1 to 5 $\mu$m) to Eq. (S16), SPP coupling coefficients $\beta_{\mathrm{t}}(\lambda)$ and $\beta_{\mathrm{b}}(\lambda)$ can be extracted (see Fig. S7). Thus, the modulation of the visibility in Fig. 4 can be theoretically predicted, provided that the visibility of the incident fields is known.

**Interference patterns calculated in Fig. 1.** The diffraction patterns in Fig. 1A–D are calculated using Eqs. (S4) and (S13). The specific input parameters are as follows: slit-slit separation distance $d = 2.3$ $\mu$m, distance between the projection screen and the plane containing the double-slits $D = 49$ $\mu$m, effective slit width $w = 545$ nm for $\lambda = 600$ nm (see Fig. S4), subtended illumination angle $\Delta\theta = 10.1°$ for panels A and B, $\Delta\theta = 15°$ for panels C and D, SPP coupling coefficients on top and bottom interfaces extracted by fitting the experimental plasmonic interferograms $\beta_{\mathrm{t}} = -0.3018 + 0.1257i$ and $\beta_{\mathrm{b}} = -0.1075 + 0.0664i$, SPP wavevectors on the two interfaces $k_{\mathrm{SPP,t}} = (1.6497 + 0.04729i) \times 10^7$ m$^{-1}$ and $k_{\mathrm{SPP,b}} = (1.0943 + 0.0023748i) \times 10^7$ m$^{-1}$.

# Supplementary Figures

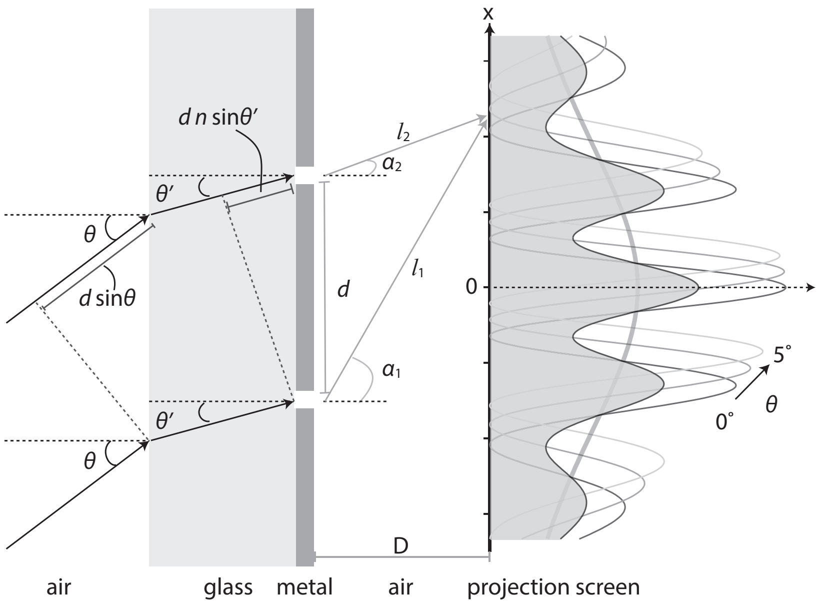


FIG. S1: **Role of angle of incidence and subtended angle in Young's double-slit interference patterns under Köhler illumination.** Under Köhler illumination, contributions to far-zone light intensity originating from linearly-polarized electromagnetic fields incident upon the sample at a given angle $\theta$ (i.e., with same wavevector) can be summed up coherently since they originate from the same point light source (thin gray lines labeled as $\theta = 0^\circ$ to $5^\circ$). In this case, the complex fields are first added, and the intensity is obtained by taking the absolute square of the total complex field amplitude. In contrast, incident light from different angles can be summed up incoherently (i.e., first the fields are calculated at each angle, the absolute square is taken, and the intensities at different angles are added up). When illuminating the double-slit interferometer with a subtended angle $\Delta\theta$ (i.e., $\theta$ varying from $-\Delta\theta/2$ to $\Delta\theta/2$), the interference pattern will be averaged out, thus resulting in reduced fringe visibility (shaded gray area). The thick gray line indicates the reference incoherent diffraction pattern, i.e., direct summation of light intensity transmitted through each slit of the double-slit interferometer.

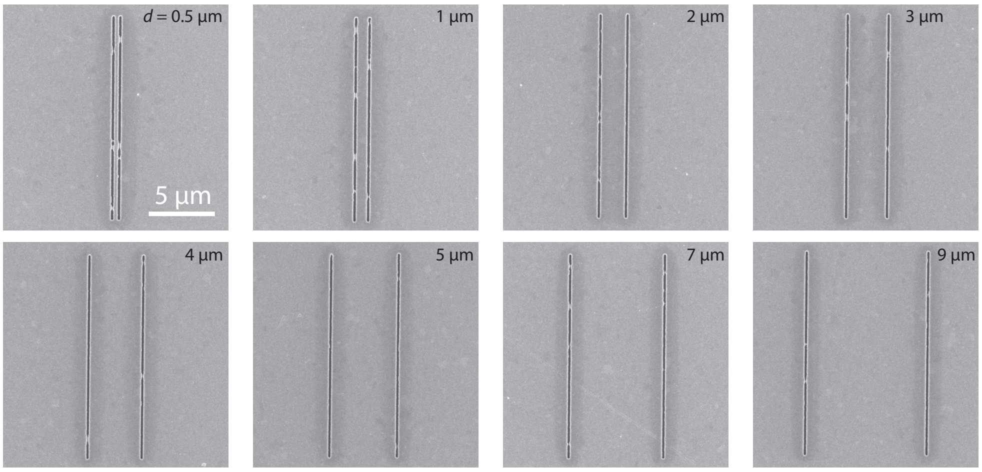


FIG. S2: **Scanning electron microscope (SEM) images of Young's double-slit interferometers.** Representative SEM images of several Young's double-slit interferometers with sub-wavelength scale widths and variable center-to-center slit-slit separation distance $d$ (with $d = 0.5, 1, 2, 3, 4, 5, 7, 9$ $\mu$m, respectively).

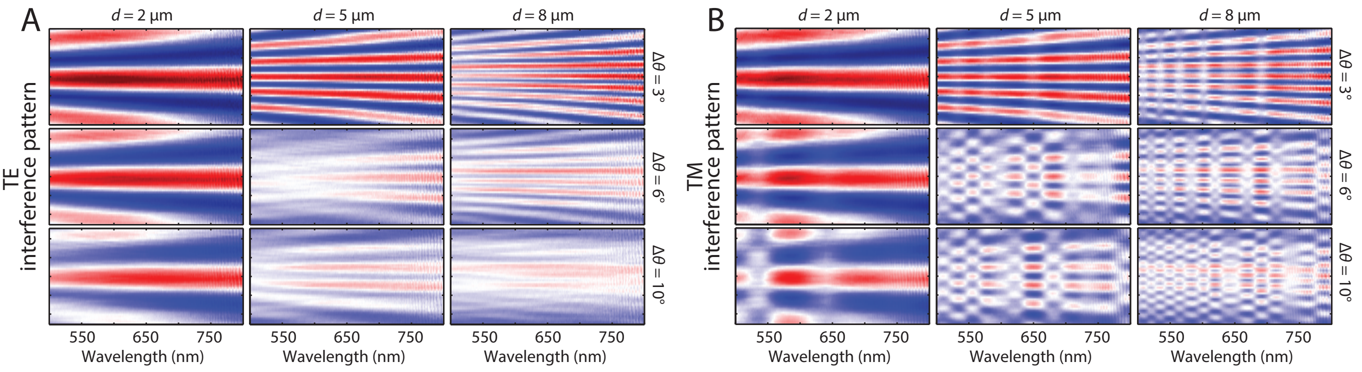


FIG. S3: **Experimental, wavelength-resolved interference patterns for representative Young's double-slit interferometers and subtended illumination angles, at two different polarizations.** Experimentally measured far-zone interference patterns originating from Young's double-slit interference, as a function of incident wavelength, for three representative double-slits ($d = 2,\ 5,\ 8\ \mu$m), three different subtended illumination angles ($\Delta\theta \approx 3°, 6°, 10°.$), and TE-(no SPPs, panel A) and TM- polarized (with SPPs, panel B) excitation.

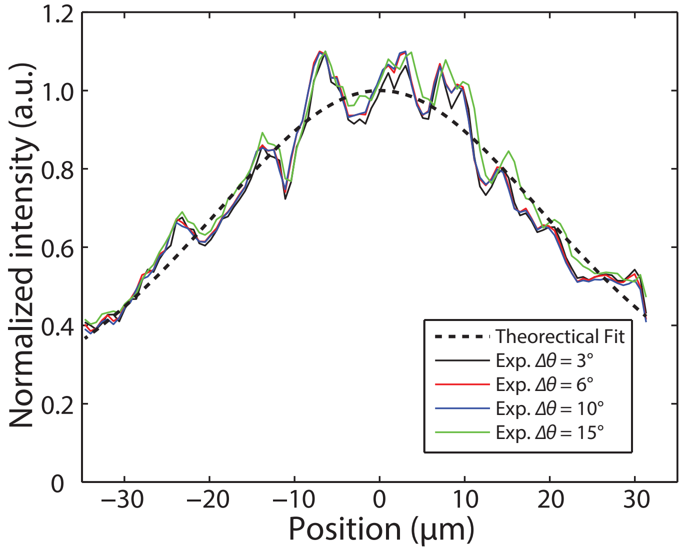


FIG. S4: **Estimate of effective optical width of individual slits.** Estimate of the effective optical slit width obtained by fitting the experimental single-slit diffraction pattern at $\lambda = 600$ nm. The mean single-slit diffraction pattern was obtained by averaging the patterns of 181 individual slits measured under Köhler illumination with a subtended angle of $\sim 3°$ at 600 nm (solid black line). Fits to the theoretical diffraction model of an individual slit in a perfectly opaque metal screen with infinitesimally small thickness lead to an estimate of the effective optical width $w = 545 \pm 12$ nm. This value is used as input parameter in the double-slit interference model to calculate the interference patterns in Fig. 1A to 1D and Figs. S1, S6, as well as the visibility curves in Fig. S5, which include the single-slit diffraction pattern from both slits. Note that because the physical width of the single slit is deeply sub-wavelength ($\sim$200 nm), the interference patterns measured under varied subtended angles (i.e., $\Delta\theta \approx 3°$, $6°$, $10°$, and $15°$) are very similar.

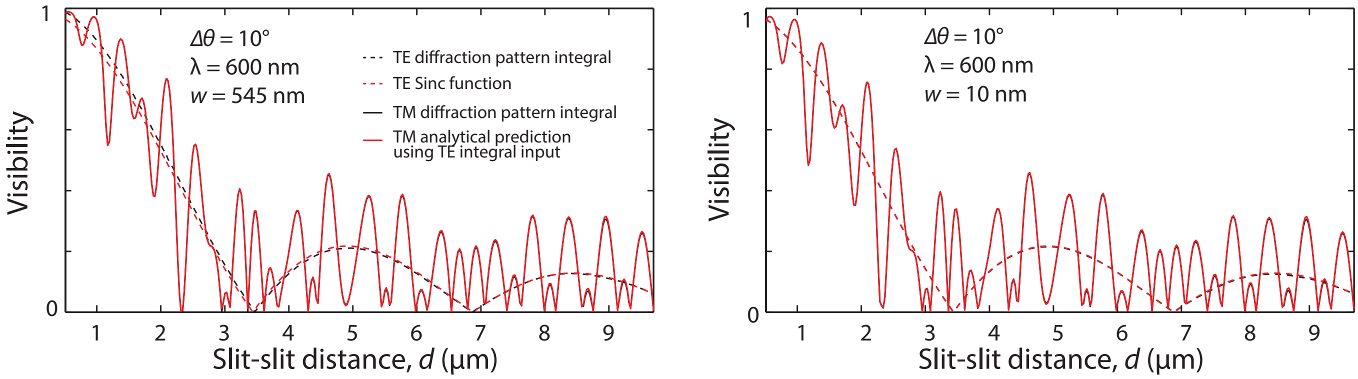


FIG. S5: **Comparison between visibility curves obtained using numerical integration and analytical expressions.** The black dashed lines and solid lines represent visibility values extracted by the numerical integration using Eqs. (S4) and (S13) for TE- and TM-polarized light illumination, respectively. The red dashed line indicates the analytical result calculated by $\mathcal{V} = |\mathrm{sinc}(k_0 d \Delta\theta/2)|$. The red solid line denotes the theoretical result obtained by using the analytical expression developed in the main text [4, 5] for TM illumination, where the input visibility values are calculated by Eq. (S4). The good agreement between dashed (solid) lines validate the analytical expression in the main text for TE(TM)-polarized illumination. Note that if an effective width $w = 545$ nm is used, only minor differences are observed for the numerical integral method and analytical equation calculations, mainly due to different intensities in the transverse propagation direction caused by single-slit diffraction. In contrast, if an effective width of 10 nm is used, the match between these two methods is improved due to the reduced difference in diffraction intensity.

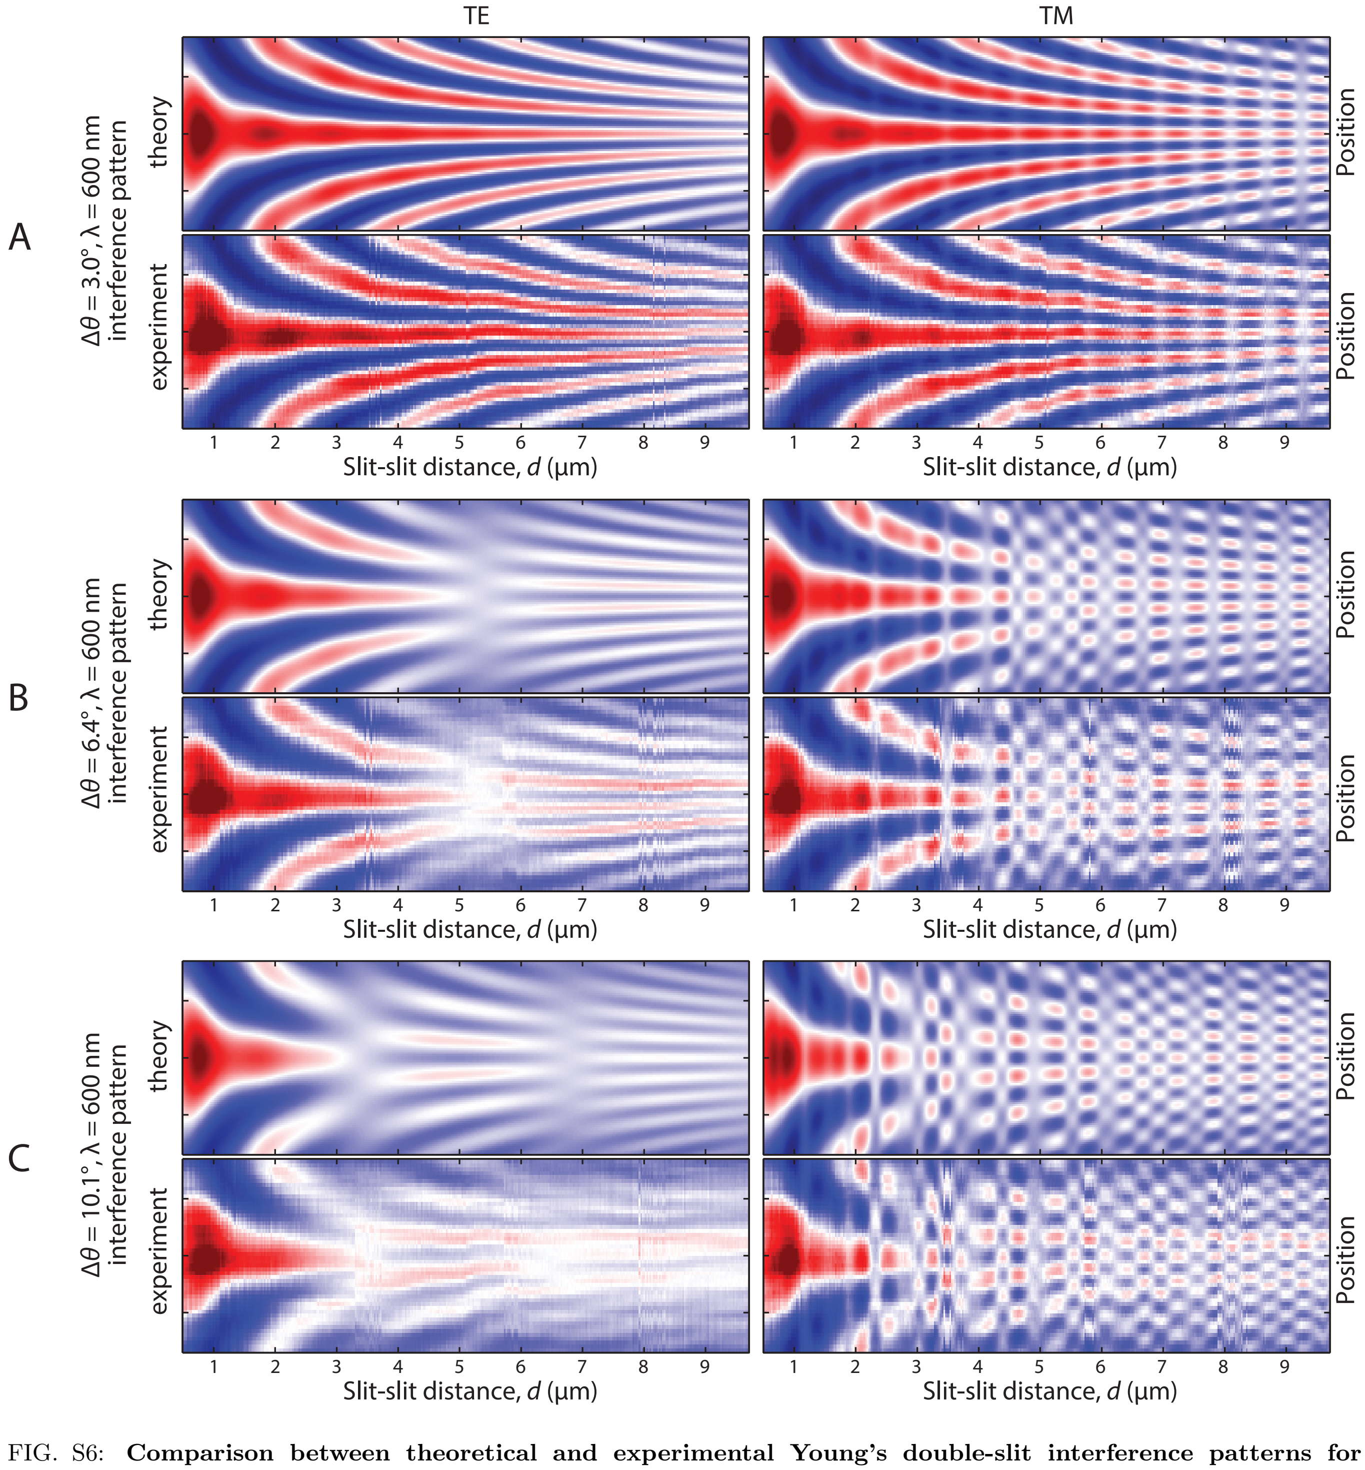


FIG. S6: **Comparison between theoretical and experimental Young's double-slit interference patterns for micrometer-scale slit-slit separation distances.** Comparison between calculated (top panels, using numerical integration of the exact theoretical model) and experimental (bottom panels) interference patterns as a function of slit-slit separation distance for various subtended angles under Köhler illumination, and for TE- (no SPPs, left panels) and TM-polarized (with SPPs, right panels) illumination conditions at wavelength $\lambda = 600$ nm. Because of the micrometer-scale slit-slit separation distances, SPP contributions become significant and cannot be neglected. Indeed, SPPs along both metal/dielectric interfaces are responsible for the observed strong modulation of fringe visibility. Theoretical results were calculated by numerically integrating the interference patterns of each angle of incidence over the whole subtended illumination angle range (from $-\Delta\theta/2$ to $\Delta\theta/2$), including SPPs on both interfaces. The agreement with the experimental data is excellent. For better quantitative comparison, both theoretical and experimental interference patterns are averaged to their mean values over the calculated/measured position range on the projection screen (i.e., -33 to 33 $\mu$m). Note that for clarity, the data plotted here cover a reduced range, i.e., from -17 to 17 $\mu$m on the projection screen.

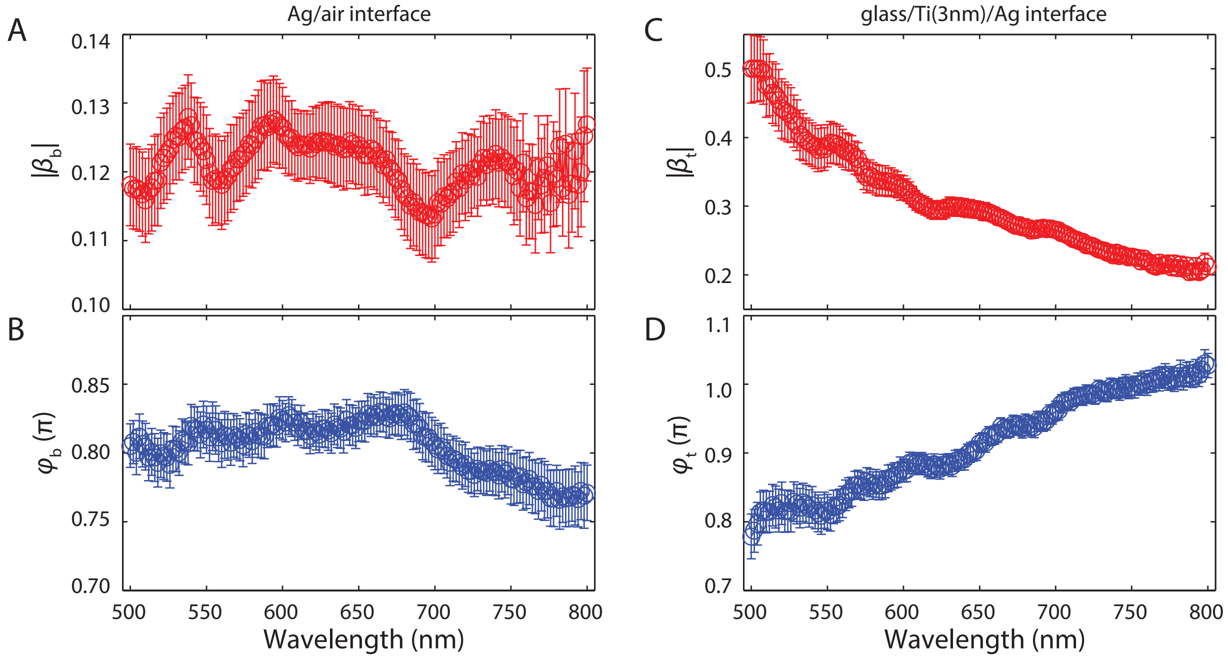


FIG. S7: **Coupling coefficients of SPPs excited along both metal/dielectric interfaces.** Amplitude ($|\beta_t|, |\beta_b|$) and phase ($\varphi_t, \varphi_b$) of SPP effective excitation coefficients (complex $\beta_t$ and $\beta_b$) as extracted from fits of the experimental plasmonic interferograms measured by directly imaging the double-slit apertures (i.e., focusing the microscope objective onto the output metal/air interface) and using a subtended illumination angle of $\Delta\theta \approx 3°$. (A, B) report the results for SPP coupling coefficients (amplitude and phase) at the Ag/air interface; (C, D) report the results for SPPs at the glass/Ti(3nm)/Ag interface. The 95% confidence intervals are also plotted.

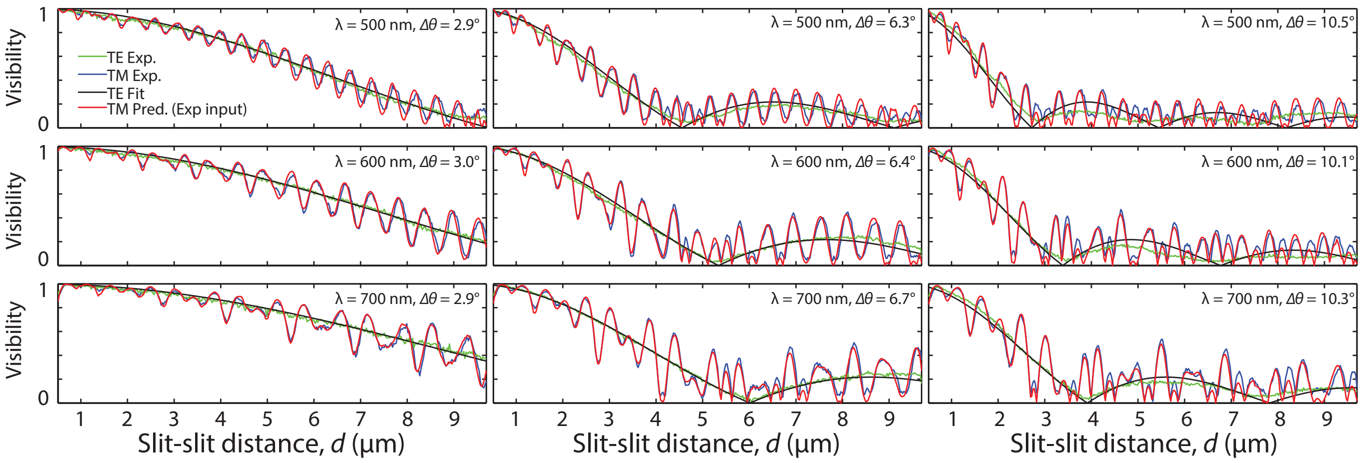


FIG. S8: **Representative visibility curves.** Experimental and simulated visibility curves as a function of slit-slit separation distance, for representative wavelengths (i.e., $\lambda = 500, 600, 700$ nm) and increasing subtended illumination angles (corresponding to decreasing spatial coherence). It is clearly seen that at short incident wavelengths (e.g., $\lambda = 500$ nm), the visibility values as a function of double-slit separation distance oscillate periodically with a single period for slit-slit separation distances larger than $\sim$3 $\mu$m. At intermediate wavelengths (e.g., 600 nm), beatings between SPPs originating from both interfaces are clearly visible for slit-slit distances smaller than 5 $\mu$m; at longer slit-slit distances, the SPP contribution from the glass/Ti(3nm)/Ag interface is attenuated and it becomes negligible, thus making the visibility oscillations single-periodic again. At longer wavelengths (e.g., 700 nm), the SPP contributions from both interfaces are responsible for significant beatings in the visibility curves all over the double-slit separation distances investigated in this work (i.e., up to $\sim$10 $\mu$m), which allow for greater visibility modulations under certain conditions.

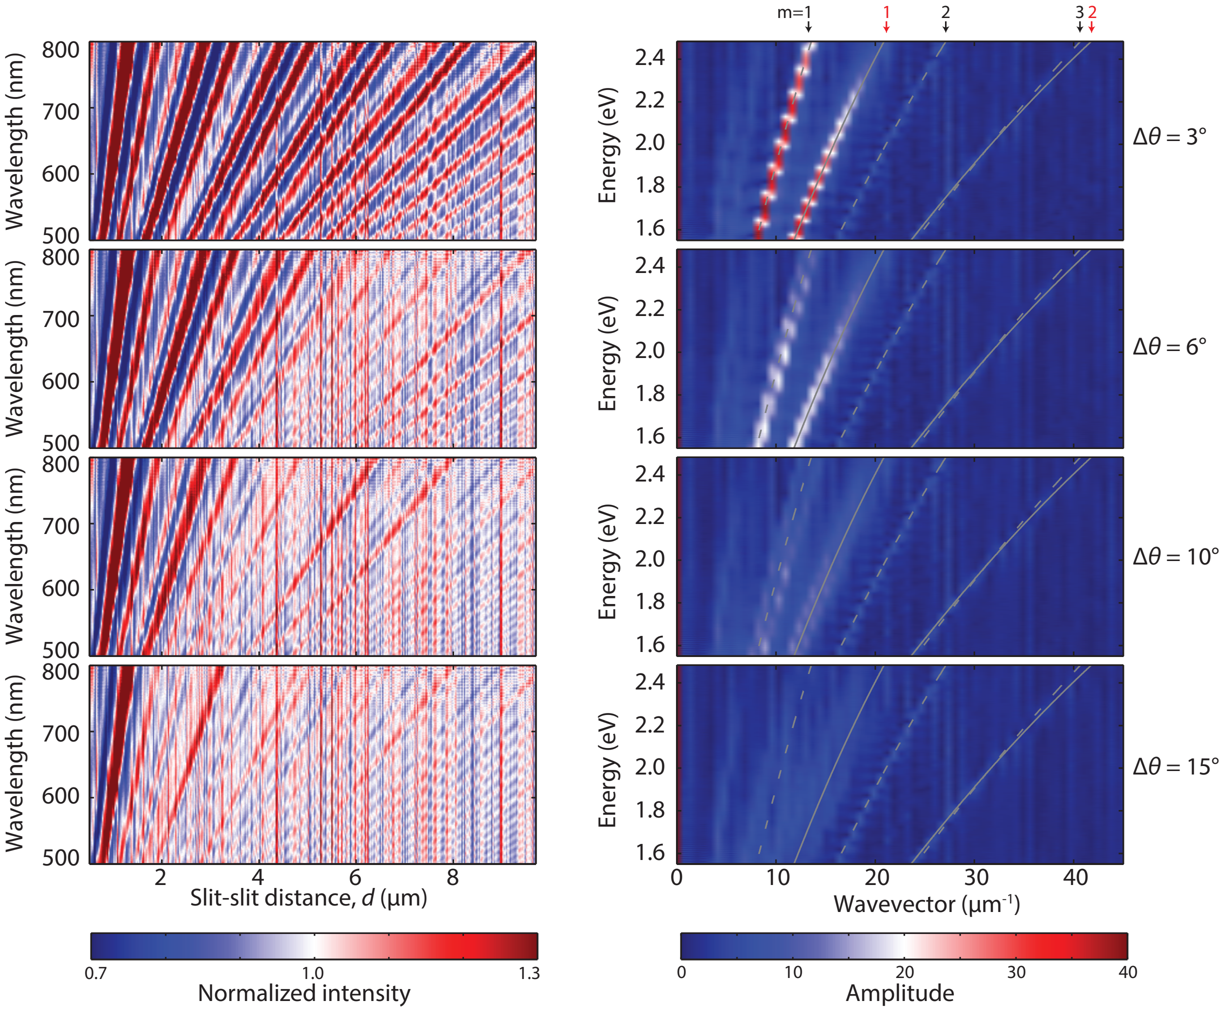


FIG. S9: **Experimental SPP energy-momentum dispersion curves.** (left panels) Wavelength-resolved plasmonic interferograms as a function of slit-slit distance and incident wavelength, and (right panels) corresponding Fourier transform power spectra that clearly show dispersion characteristics of SPPs excited and propagate along the two metal/dielectric interfaces, i.e., Ag/air ($m$ = 1, 2, 3, black labels and dashed gray lines) and glass/Ti/Ag ($m$ = 1, 2, red labels and solid gray lines). When the spatial coherence of the incidence light beam is reduced, the first-order SPP interference effects are almost entirely suppressed.

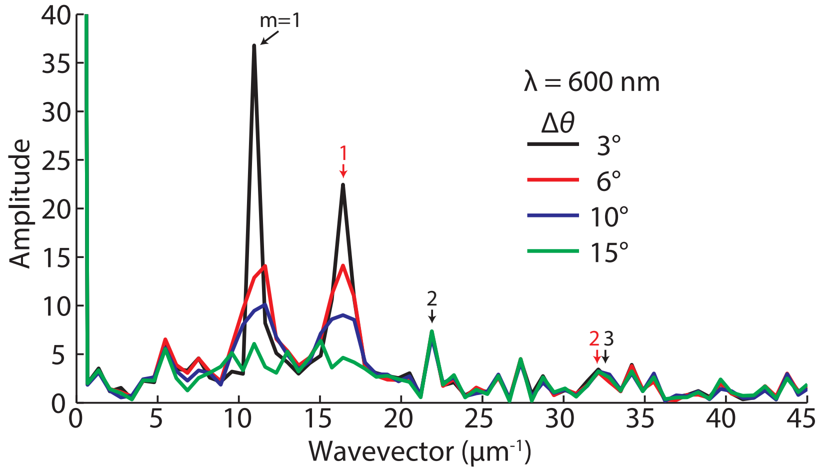


FIG. S10: **Fourier transform analysis.** Discrete Fourier transform power spectra for four different subtended illumination angles ($\Delta\theta \approx 3^\circ, 6^\circ, 10^\circ, 15^\circ$) at a specific wavelength $\lambda = 600$ nm. The data clearly shows the first-order SPP contributions at the two interfaces, characterized by different wavevectors. Also, the first-order SPP contributions can be significantly suppressed for large subtended Köhler illumination angles $\Delta\theta$. However, it is worth noting that, differently from the case of plasmonic interferograms, the first-order SPP contributions always dominate the SPP-assisted modulation of spatial coherence even for large $\Delta\theta$. Indeed, light directly transmitted through one slit can always interfere with a fraction of light transmitted through the other slit that is originally generated by scattering at the first slit, followed by SPP generation, propagation toward the second slit, and scattering back into free space through the second slit.

[1] D. Morrill, D. Li, and D. Pacifici, Nat. Photonics **10**, 681 (2016).
[2] P. Lüsse, P. Stuwe, J. Schüle, and H.-G. Unger, J. Lightwave Technology **12**, 487 (1994).
[3] A. D. Rakic, A. B. Djurišic, J. M. Elazar, and M. L. Majewski, Appl. Opt. **37**, 5271 (1998).
[4] C. H. Gan, G. Gbur, and T. D. Visser, Phys. Rev. Lett. **98**, 043908 (2007).
[5] S. Divitt, M. Frimmer, T. D. Visser, and L. Novotny, Optics Lett. **41**, 3094 (2016).
[6] D. Li, J. Feng, and D. Pacifici, Opt. Express **24**, 27309 (2016).
